# Supplementary material for: Incremental Calibration of Architectural Performance Models with Parametric Dependencies
Source: arXiv:2006.16953 source file (2020-06-30)
Supplement: Supplementary file 1 [file Appendix.tex]

\section{Appendix}
\label{appendix}

\subsection{Additional Evaluation Results}

\begin{table}[H]
    \centering
    \begin{tabular}{|c|c|c|c|}
    \hline 
    Measure & Monitoring & Analysis \\ \hline \hline
    Avg. Response Time & 172.97ms & 136.30ms \\ \hline
    Avg. KS-Test & -- & \cocomeavg \\ \hline
    Avg. Wasserstein Distance & -- & 23.9742 \\ \hline
    \end{tabular}
    \caption{Aggregated measurements and metrics (across 100 repetitions) about the calibration accuracy for CoCoME's "bookSale" service}
    \label{table:cocome:metrics}
\end{table}

\begin{figure}[H]
\centering
\begin{tikzpicture}
\begin{axis}[
    xlabel={Repetition number},
    ylabel={WS-Distance},
    xmin=1, xmax=100,
    ymin=0, ymax=100,
    xtick={0, 25, 50, 75, 100},
    ytick={0, 20, 40, 60, 80, 100},
    legend style={
        at={(0.5,-0.2)},
        anchor=north,
        legend columns=-1
      },
    ymajorgrids=true,
    grid style=dashed,
]

\addplot[
    color=red,
    mark=point,
    ]
    coordinates {
    (1,22.400235474353163)(2,23.533760780753546)(3,29.805591806627344)(4,17.853977530640048)(5,24.98883624602816)(6,25.95961472991379)(7,31.3685315478893)(8,18.876134816159787)(9,22.927726395823896)(10,24.052201543349984)(11,19.954805946436704)(12,24.572443826600107)(13,17.261192124375867)(14,24.155937925556078)(15,24.049109169314594)(16,28.005915229232645)(17,30.92310201997254)(18,17.051662505674095)(19,18.049293576940553)(20,21.87515603722199)(21,24.855495347253765)(22,16.398079323649583)(23,27.954961983658666)(24,29.27549080798914)(25,24.505858488424895)(26,24.800541874716313)(27,34.44815308670006)(28,35.20399738992307)(29,14.583933840217892)(30,27.419328756241555)(31,19.903483885610548)(32,15.82261404902407)(33,37.52036995006813)(34,25.15569677712213)(35,17.60226112119837)(36,19.612176577394496)(37,25.03381752156152)(38,22.190932818883436)(39,24.187627666817995)(40,30.293591125737652)(41,23.896802655469827)(42,23.6891880390377)(43,31.16948479346354)(44,16.93010950975943)(45,22.040966863368148)(46,20.425314911484357)(47,23.19506071266457)(48,41.23836813436231)(49,20.998326146164345)(50,18.941769745801246)(51,22.92362687244668)(52,22.37119836586475)(53,21.37230481162054)(54,23.13060315478894)(55,22.54618701770314)(56,32.49997162959603)(57,29.432435882887003)(58,19.118176917839335)(59,23.92372616886066)(60,22.03323592827966)(61,16.67161257376307)(62,19.720977076713595)(63,20.92575465274627)(64,25.107467090331415)(65,24.19423797094872)(66,32.7148206990468)(67,20.162307081252866)(68,27.23337494325921)(69,21.696706196096265)(70,21.911257376305052)(71,20.290456196096216)(72,15.419115978211579)(73,23.6750879482524)(74,31.62620574216979)(75,22.257291193826607)(76,27.953231389015052)(77,23.36118361325467)(78,31.250836926917867)(79,16.861481502496616)(80,21.294513163867475)(81,17.381808896958713)(82,22.016554130730828)(83,30.575649682251512)(84,23.516015093054936)(85,18.41856275533366)(86,23.902278143440792)(87,21.342913073082187)(88,25.584033136631884)(89,24.672080685429005)(90,28.68883340898777)(91,20.86794995460737)(92,36.17198138901508)(93,29.734694167044996)(94,17.041122900590118)(95,20.776909328188854)(96,31.736311280072655)(97,17.81177655469816)(98,31.200082274171606)(99,24.097650930549268)(100,21.252723558783494)
    };

\end{axis}
\end{tikzpicture}
\caption{Absolute Wasserstein distance (between the monitoring and the simulation results) for CoCoME's "bookSale" service (100 simulation repetitions)}
\label{fig:ws:booksale}
\end{figure}

\begin{figure}[!h]
\centering
\begin{tikzpicture}
\begin{axis}[
    xlabel={Repetition number},
    ylabel={WS-Distance},
    xmin=1, xmax=100,
    ymin=0, ymax=100,
    xtick={0, 25, 50, 75, 100},
    ytick={0, 20, 40, 60, 80, 100},
    legend columns=1, 
    legend style={
        at={(0.5,-0.2)},
        anchor=north,
        legend columns=-1
      },
    ymajorgrids=true,
    grid style=dashed,
]

\addplot[
    color=red,
    mark=point,
    ]
    coordinates {
    (1,11.4761597782)(2,17.1864331372)(3,16.3622733106)(4,21.3752814702)(5,22.2351728772)(6,13.9468929324)(7,19.2004491417)(8,15.9770193216)(9,12.6300664633)(10,19.0606976829)(11,20.7657320646)(12,22.3886074187)(13,16.6082185536)(14,26.147093896)(15,13.3164501319)(16,19.6056057965)(17,38.7047165928)(18,23.2561560253)(19,23.600602891)(20,22.1096583618)(21,22.0906485315)(22,14.9401769933)(23,16.9117212658)(24,15.050573836)(25,21.2579114307)(26,19.5240097092)(27,12.1955569666)(28,17.6341735067)(29,24.4929874579)(30,29.255054357)(31,15.7042777415)(32,14.747200431)(33,26.7931769207)(34,12.8132339411)(35,27.3452004794)(36,19.5581583981)(37,20.8486931309)(38,16.4945975884)(39,25.4381532676)(40,19.6783612988)(41,18.6652169439)(42,23.6265011743)(43,14.4261730951)(44,8.5752524152)(45,19.6020616934)(46,18.7476937604)(47,9.63149197356)(48,27.5222694366)(49,16.2128308031)(50,22.8214964529)(51,15.0624833539)(52,21.2959220116)(53,24.6067589162)(54,15.5483341808)(55,12.8507300065)(56,26.9684541537)(57,11.8014666715)(58,21.4725036924)(59,19.9301167042)(60,10.7575875887)(61,21.0361462192)(62,20.8325615603)(63,12.8457301276)(64,19.1016107358)(65,24.6772491941)(66,15.0907181424)(67,28.5389094695)(68,17.6162441587)(69,21.5400414034)(70,20.2867333721)(71,21.9357249219)(72,22.9260732186)(73,7.74519684753)(74,20.4383519769)(75,22.4123053921)(76,21.790107779)(77,13.2395856033)(78,11.5306608381)(79,18.240911237)(80,17.7961459771)(81,20.285368393)(82,22.6505956272)(83,20.5447719184)(84,11.2035150481)(85,16.3687531779)(86,18.792078279)(87,25.1097098133)(88,24.349168301)(89,20.9223021234)(90,26.8905171788)(91,12.4601771352)(92,14.5047547275)(93,19.7193439626)(94,17.0464244207)(95,22.3562716399)(96,15.5109137793)(97,18.4219903876)(98,15.4320415971)(99,20.1538491804)(100,26.4449220149)
    };
    
\addplot[
    color=blue,
    mark=point,
    ]
    coordinates {
    (1,11.7211237016)(2,13.3997167139)(3,19.6135096003)(4,10.7261525361)(5,27.6297733711)(6,14.533578848)(7,27.7996467355)(8,16.9120428077)(9,20.6799276047)(10,9.02589167376)(11,9.55769996231)(12,9.99842933585)(13,18.1826782606)(14,15.4124974707)(15,20.0331971951)(16,21.968533645)(17,13.9508254081)(18,23.8221167343)(19,17.047349701)(20,12.3204658483)(21,14.9526156752)(22,13.5137638271)(23,14.4468319169)(24,11.5511000944)(25,47.1203808624)(26,16.3295730473)(27,12.6633743086)(28,18.6015926975)(29,18.3100094429)(30,14.108470255)(31,10.4738505528)(32,19.5774441297)(33,18.1872033365)(34,15.4621372364)(35,8.31793573767)(36,15.4208569405)(37,13.6618711281)(38,15.5467831287)(39,9.26375118036)(40,12.8995996308)(41,15.660877086)(42,9.49950897073)(43,23.612625118)(44,32.8779540447)(45,14.480166824)(46,13.8925007869)(47,34.0630395926)(48,9.67785961599)(49,16.2652754171)(50,15.6748027115)(51,14.8136323576)(52,10.4490368272)(53,35.0549077634)(54,9.36571608436)(55,10.8969255622)(56,18.1767485049)(57,11.4700881335)(58,10.7233660461)(59,16.8395133549)(60,12.9550620531)(61,9.38974346868)(62,20.8997450425)(63,35.7554831602)(64,15.6477387697)(65,11.2811646777)(66,10.8841989298)(67,14.3127824992)(68,7.50786203292)(69,15.4882530689)(70,12.8034592383)(71,40.6581586402)(72,14.3256858785)(73,17.6215832546)(74,17.5433805477)(75,13.4643404027)(76,10.7482562166)(77,14.7706014771)(78,8.3344916588)(79,7.5253604029)(80,14.2851872836)(81,10.3704910293)(82,11.1503273528)(83,15.1672526305)(84,15.0885269122)(85,12.9495624803)(86,19.7756468366)(87,18.6955944562)(88,21.6379697828)(89,22.3682294618)(90,12.8022350938)(91,7.05833080399)(92,6.41622757318)(93,23.7510387158)(94,20.8233931382)(95,13.6602210643)(96,15.7138641576)(97,10.6017437834)(98,10.1722818022)(99,12.0888936665)(100,41.9648253069)
    };
    
\addplot[
    color=orange,
    mark=point,
    ]
    coordinates {
    (1,25.3090544493)(2,32.9394357519)(3,30.6337210736)(4,37.1035970798)(5,31.6835019308)(6,43.1217326215)(7,29.2349227915)(8,36.1797371561)(9,43.8389700434)(10,45.981468182)(11,33.6213341462)(12,23.4718563046)(13,32.939020183)(14,54.0275334941)(15,25.8850122754)(16,41.5485537148)(17,33.188985356)(18,48.0545309885)(19,28.5184878542)(20,42.4196180049)(21,48.1444170885)(22,29.2220906753)(23,39.2104347514)(24,43.8852790629)(25,34.8347955745)(26,48.0676106021)(27,38.0249933013)(28,32.0934973046)(29,34.5771528218)(30,54.7241841919)(31,47.6656869252)(32,48.6958832225)(33,37.9761175451)(34,25.4555578152)(35,41.5316927443)(36,40.3276493244)(37,42.5132714208)(38,43.6435780947)(39,27.7717099259)(40,51.1439621236)(41,44.3057627773)(42,48.1157924996)(43,38.0616811218)(44,39.1864881407)(45,49.4110810737)(46,46.8049378739)(47,46.9334263946)(48,33.7168899226)(49,35.4579303109)(50,30.4688665976)(51,22.4151286478)(52,45.3882924273)(53,49.2434095434)(54,26.7430693765)(55,42.5445964829)(56,45.7683540488)(57,41.3877274824)(58,51.865684154)(59,51.9678558451)(60,50.2271866851)(61,38.9688742702)(62,54.3026622013)(63,41.8674604596)(64,34.9787429083)(65,27.626685627)(66,36.9684479532)(67,53.1160488149)(68,29.4636512133)(69,28.9049741593)(70,38.358002144)(71,33.0515227865)(72,50.7465999112)(73,28.5519764472)(74,45.948279871)(75,48.6437948588)(76,51.7150052398)(77,50.0416537696)(78,39.5437577937)(79,33.5807278611)(80,43.7003973467)(81,28.9292143283)(82,38.6164030146)(83,54.9709553714)(84,46.7334464139)(85,34.0723943112)(86,53.9110801591)(87,46.4014378181)(88,27.9972092254)(89,36.2220508244)(90,44.7125140662)(91,44.6895282249)(92,35.260881427)(93,34.47384755)(94,26.1906736444)(95,33.9798598967)(96,36.0366998474)(97,49.1969354264)(98,49.0281277803)(99,30.3322078157)(100,30.3247136646)
    };    
    
\addplot[
    color=green,
    mark=point,
    ]
    coordinates {
   (1,56.6857646878)(2,71.4571732628)(3,46.2849459273)(4,35.4814278775)(5,58.6944976223)(6,57.2981006801)(7,49.4283433864)(8,41.0862451515)(9,55.0388983484)(10,52.9693429463)(11,54.4956897786)(12,56.6825640436)(13,42.5099856829)(14,48.42394718)(15,31.7028445697)(16,56.2266349645)(17,40.468220586)(18,51.4903297778)(19,31.3374794191)(20,46.458759286)(21,45.1711637777)(22,58.9283264304)(23,29.4039538273)(24,46.7443199366)(25,64.031350156)(26,66.5468411018)(27,47.7560119139)(28,67.2713588485)(29,66.5353538375)(30,36.3585644526)(31,37.7645732172)(32,67.5082362271)(33,61.8623546556)(34,41.103537325)(35,37.5917382523)(36,44.1987480277)(37,39.6385181776)(38,56.8739960117)(39,30.6830475526)(40,63.9841179629)(41,43.8744958327)(42,60.216687348)(43,36.8310456614)(44,44.0836524555)(45,51.2727713497)(46,49.8033721941)(47,79.2013795572)(48,59.8207048627)(49,54.0471677569)(50,42.7601216956)(51,44.8144375415)(52,54.638276215)(53,59.0770800736)(54,50.1948261127)(55,34.0768387278)(56,45.8184064986)(57,62.2562616966)(58,46.049571445)(59,61.6951045661)(60,59.0917712328)(61,51.7395722759)(62,46.4218083039)(63,69.9359468477)(64,51.0873025004)(65,54.3819028992)(66,44.2713043923)(67,67.3475260502)(68,62.1293846193)(69,56.0840952089)(70,30.0864575344)(71,62.1851579449)(72,58.4361185253)(73,40.4310643248)(74,71.3627225901)(75,42.2522961088)(76,69.3542440504)(77,24.2525536618)(78,52.1571690443)(79,58.0090679229)(80,46.9223682058)(81,53.4165805083)(82,55.4886391062)(83,50.9076149205)(84,62.1324129468)(85,20.8585242514)(86,33.4808666973)(87,67.8850368155)(88,54.5639668661)(89,55.5467911745)(90,60.6727120724)(91,39.5266612977)(92,49.9140563481)(93,46.203664289)(94,61.8925202156)(95,60.8622666163)(96,36.6332151208)(97,67.3921641867)(98,41.304701897)(99,65.7374290535)(100,58.2486904945)
    };    
    
\legend{Parameterized (20 Users), Non-Parameterized (20 Users), Parameterized (40 Users), Non-Parameterized (40 Users)}

\end{axis}
\end{tikzpicture}
\caption{Comparison of the Wasserstein distances for the "train" service (100 simulation repetitions)}
\label{fig:comp:ws:train}
\end{figure}

\begin{table}[H]
    \centering
    \begin{tabular}{|c|c|c|c|}
    \hline 
    Measure & Monitoring & PM & NPM \\ \hline \hline
    Avg. Response Time & 94.92ms & 86.62ms & 102.25ms \\ \hline
    Avg. KS-Test & -- & 0.1267 & 0.1239 \\ \hline
    Avg. Wasserstein Distance & -- & 19.1764 & 16.2669 \\ \hline
    \end{tabular}
    \caption*{PM=Parameterized Model, NPM=Non-Parameterized Model}
    \caption{Aggregated measurements and metrics (across 100 repetitions) about the calibration accuracy for TeaStore's "train" service using a load of \textbf{20 users}}
    \label{table:teastore:param:20}
\end{table}

\begin{table}[H]
    \centering
    \begin{tabular}{|c|c|c|c|}
    \hline 
    Measure & Monitoring & PM & NPM \\ \hline \hline
    Avg. Response Time & 154.19ms & 184.85ms & 103.87ms \\ \hline
    Avg. KS-Test & -- & 0.1609 & 0.2575 \\ \hline
    Avg. Wasserstein Distance & -- & 39.6138 & 51.3531 \\ \hline
    \end{tabular}
    \caption*{PM=Parameterized Model, NPM=Non-Parameterized Model}
    \caption{Aggregated measurements and metrics (across 100 repetitions) about the calibration accuracy for TeaStore's "train" service using a load of \textbf{40 users}}
    \label{table:teastore:param:40}
\end{table}
